# Supplementary material for: Analyzing Differentiable Fuzzy Logic Operators
Source: arXiv:2002.06100 source file (2021-08-24)
Supplement: Supplementary file 1 [file appendix_rules.tex]

\begin{table}[h]
\begin{tabular}{l|l|l|l|l}
\hline
Formula & $a, c$ & $\neg a, c$ & $a, \neg c$ & $\neg a, \neg c$ \\ \hline

\specialcell{ $\forall x_0,x_1\ \pred{drawer}(x_0) \wedge \pred{cHas}(x_0, x_1) \rightarrow \pred{handle}(x_1)$} & 59 & 2223 & 1 & 614641 \\ \hline
\specialcell{ $\forall x_0,x_1\ \pred{house}(x_0) \wedge \pred{cHas}(x_0, x_1) \rightarrow \pred{window}(x_1) \vee \pred{roof}(x_1) \vee $ \\ $\pred{door}(x_1)$} & 378 & 28311 & 23 & 588212 \\ \hline
\specialcell{ $\forall x_0,x_1\ \pred{trunk}(x_0) \wedge \pred{on}(x_0, x_1) \rightarrow \pred{elephant}(x_1) \vee \pred{tree}(x_1)$} & 248 & 22794 & 44 & 593838 \\ \hline
\specialcell{ $\forall x_0,x_1\ \pred{in}(x_0, x_1) \wedge \pred{leaf}(x_0) \rightarrow \pred{flower}(x_1) \vee \pred{tree}(x_1) \vee $ \\ $\pred{vase}(x_1) \vee \pred{pot}(x_1)$} & 310 & 23124 & 41 & 593449 \\ \hline
\specialcell{ $\forall x_0,x_1\ \pred{head}(x_0) \wedge \pred{cHas}(x_0, x_1) \rightarrow \pred{headHas}(x_1)$} & 289 & 35932 & 37 & 580666 \\ \hline
\specialcell{ $\forall x_0,x_1\ \pred{autos}(x_0) \wedge \pred{cHas}(x_0, x_1) \rightarrow \pred{autosHas}(x_1)$} & 2184 & 63890 & 174 & 550676 \\ \hline
\specialcell{ $\forall x_0,x_1\ \pred{planes}(x_0) \wedge \pred{cHas}(x_0, x_1) \rightarrow \pred{planesHas}(x_1)$} & 1796 & 53408 & 35 & 561685 \\ \hline
\specialcell{ $\forall x_0,x_1\ \pred{glass}(x_0) \wedge \pred{on}(x_0, x_1) \rightarrow \pred{glassOn}(x_1)$} & 2215 & 216458 & 77 & 398174 \\ \hline
\specialcell{ $\forall x_0,x_1\ \pred{structure}(x_0) \wedge \pred{cHas}(x_0, x_1) \rightarrow \pred{structureHas}(x_1)$} & 3401 & 56894 & 117 & 556512 \\ \hline
\specialcell{ $\forall x_0,x_1\ \pred{snow}(x_0) \wedge \pred{on}(x_0, x_1) \rightarrow \pred{outsideStationary}(x_1)$} & 958 & 129370 & 116 & 486480 \\ \hline
\specialcell{ $\forall x_0,x_1\ \pred{snow}(x_0) \wedge \pred{cHas}(x_0, x_1) \rightarrow \pred{track}(x_1)$} & 114 & 3999 & 54 & 612757 \\ \hline
\specialcell{ $\forall x_0,x_1\ \pred{sign}(x_0) \wedge \pred{on}(x_0, x_1) \rightarrow \pred{signsOn}(x_1)$} & 3880 & 116611 & 320 & 496113 \\ \hline
\specialcell{ $\forall x_0,x_1\ \pred{basket}(x_0) \wedge \pred{on}(x_0, x_1) \rightarrow \pred{basketOn}(x_1)$} & 256 & 36761 & 45 & 579862 \\ \hline
\specialcell{ $\forall x_0,x_1\ \pred{pole}(x_0) \wedge \pred{cHas}(x_0, x_1) \rightarrow \pred{onPole}(x_1)$} & 411 & 30215 & 30 & 586268 \\ \hline
\specialcell{ $\forall x_0,x_1\ \pred{tree}(x_0) \wedge \pred{on}(x_0, x_1) \rightarrow \pred{treeOn}(x_1)$} & 1005 & 67832 & 87 & 548000 \\ \hline
\specialcell{ $\forall x_0,x_1\ \pred{hair}(x_0) \wedge \pred{growing on}(x_0, x_1) \rightarrow \pred{placesForHair}(x_1)$} & 10 & 48016 & 0 & 568898 \\ \hline
\specialcell{ $\forall x_0,x_1\ \pred{fruits}(x_0) \wedge \pred{growing on}(x_0, x_1) \rightarrow \pred{tree}(x_1)$} & 8 & 17285 & 0 & 599631 \\ \hline
\specialcell{ $\forall x_0,x_1\ \pred{curtain}(x_0) \wedge \pred{on}(x_0, x_1) \rightarrow \pred{curtainOn}(x_1)$} & 366 & 29435 & 13 & 587110 \\ \hline
\specialcell{ $\forall x_0,x_1\ \pred{engine}(x_0) \wedge \pred{related}(x_0, x_1) \rightarrow \pred{transport}(x_1) \vee $ \\ $\pred{wing}(x_1)$} & 1014 & 45141 & 62 & 570707 \\ \hline
\specialcell{ $\forall x_0,x_1\ \pred{in}(x_0, x_1) \rightarrow \pred{thingsIn}(x_1)$} & 17024 & 220867 & 3510 & 375523 \\ \hline
\specialcell{ $\forall x_0,x_1\ \pred{on}(x_0, x_1) \rightarrow \pred{thingsOn}(x_1)$} & 32808 & 42217 & 69035 & 472864 \\ \hline
\specialcell{ $\forall x_0,x_1\ \pred{covered in}(x_0, x_1) \rightarrow \pred{snow}(x_1) \vee \pred{leaf}(x_1) \vee \pred{tree}(x_1) \vee $ \\ $\pred{food}(x_1)$} & 408 & 31066 & 26 & 585424 \\ \hline
\specialcell{ $\forall x_0,x_1\ \pred{covering}(x_0, x_1) \wedge \pred{human}(x_0) \vee \pred{hand}(x_0) \rightarrow \pred{face}(x_1) \vee $ \\ $\pred{head}(x_1) \vee \pred{ear}(x_1) \vee \pred{mouth}(x_1)$} & 16 & 23727 & 1 & 593180 \\ \hline
\specialcell{ $\forall x_0,x_1\ \pred{riding}(x_0, x_1) \rightarrow \pred{ridingOn}(x_1)$} & 3045 & 61185 & 41 & 552653 \\ \hline
\specialcell{ $\forall x_0,x_1\ \pred{walking}(x_0, x_1) \rightarrow \pred{placesToWalkOn}(x_1)$} & 1610 & 27022 & 62 & 588230 \\ \hline
\specialcell{ $\forall x_0,x_1\ \pred{hold}(x_0, x_1) \rightarrow \pred{thingsToHold}(x_1)$} & 8990 & 215029 & 395 & 392510 \\ \hline
\end{tabular}
\caption{The first set of rules for the Visual Genome dataset.}
\label{table:vs_rules1}
\end{table}
\begin{table}[]
\begin{tabular}{l|l|l|l|l}
\hline
Formula & $a, c$ & $\neg a, c$ & $a, \neg c$ & $\neg a, \neg c$ \\ \hline
\specialcell{ $\forall x_0,x_1\ \pred{sitting on}(x_0, x_1) \rightarrow \pred{thingsToSitOn}(x_1)$} & 3545 & 104337 & 764 & 508278 \\ \hline
\specialcell{ $\forall x_0,x_1\ \pred{hair}(x_1) \wedge \pred{cHas}(x_0, x_1) \rightarrow \pred{human}(x_0) \vee \pred{animals}(x_0) \vee $ \\ $\pred{tail}(x_0)$} & 5735 & 166510 & 154 & 444525 \\ \hline
\specialcell{ $\forall x_0,x_1\ \pred{window}(x_1) \wedge \pred{cHas}(x_0, x_1) \rightarrow \pred{house}(x_0) \vee \pred{building}(x_0) \vee $ \\ $\pred{transport}(x_0) \vee \pred{door}(x_0)$} & 3250 & 68870 & 157 & 544647 \\ \hline
\specialcell{ $\forall x_0,x_1\ \pred{bodypart}(x_1) \wedge  \neg \pred{specialBodyparts}(x_1) \wedge \pred{cHas}(x_0, x_1) \rightarrow $ \\ $\pred{animals}(x_0) \vee \pred{human}(x_0)$} & 17800 & 149555 & 763 & 448806 \\ \hline

\specialcell{ $\forall x_0,x_1\ \pred{bodypartAnimal}(x_1) \wedge  \neg \pred{specialBodyparts}(x_1) \wedge $ \\ $\pred{cHas}(x_0, x_1) \rightarrow \pred{animals}(x_0)$} & 633 & 43460 & 17 & 572814 \\ \hline
\specialcell{ $\forall x_0,x_1\ \pred{arm}(x_1) \wedge \pred{cHas}(x_0, x_1) \rightarrow \pred{hasArm}(x_0)$} & 1852 & 137418 & 40 & 477614 \\ \hline
\specialcell{ $\forall x_0,x_1\ \pred{tail}(x_1) \wedge \pred{cHas}(x_0, x_1) \rightarrow \pred{hasTail}(x_0)$} & 2380 & 49140 & 15 & 565389 \\ \hline
\specialcell{ $\forall x_0,x_1\ \pred{leg}(x_1) \wedge \pred{cHas}(x_0, x_1) \rightarrow \pred{hasLeg}(x_0)$} & 4803 & 193375 & 52 & 418694 \\ \hline
\specialcell{ $\forall x_0,x_1\ \pred{face}(x_1) \wedge \pred{cHas}(x_0, x_1) \rightarrow \pred{hasFace}(x_0)$} & 1701 & 189445 & 60 & 425718 \\ \hline
\specialcell{ $\forall x_0,x_1\ \pred{flower}(x_1) \wedge \pred{in}(x_0, x_1) \rightarrow \pred{leaf}(x_0) \vee \pred{flower}(x_0) \vee $ \\ $\pred{vase}(x_0)$} & 31 & 9931 & 11 & 606951 \\ \hline
\specialcell{ $\forall x_0,x_1\ \pred{tree}(x_1) \wedge \pred{in}(x_0, x_1) \rightarrow \pred{leaf}(x_0) \vee \pred{bird}(x_0) \vee \pred{tree}(x_0) \vee $ \\ $\pred{branch}(x_0) \vee \pred{banana}(x_0)$} & 375 & 28572 & 269 & 587708 \\ \hline
\specialcell{ $\forall x_0,x_1\ \pred{counter}(x_1) \wedge \pred{in}(x_0, x_1) \rightarrow \pred{sink}(x_0) \vee \pred{drawer}(x_0)$} & 75 & 1937 & 15 & 614897 \\ \hline
\specialcell{ $\forall x_0,x_1\ \pred{human}(x_1) \wedge \pred{on}(x_0, x_1) \rightarrow \pred{onHuman}(x_0)$} & 9513 & 121859 & 327 & 485225 \\ \hline
\specialcell{ $\forall x_0,x_1\ \pred{window}(x_1) \wedge \pred{cHas}(x_0, x_1) \rightarrow \pred{hasWindow}(x_0)$} & 3299 & 65235 & 108 & 548282 \\ \hline
\specialcell{ $\forall x_0,x_1\ \pred{pole}(x_1) \wedge \pred{on}(x_0, x_1) \rightarrow \pred{onPole}(x_0)$} & 2654 & 27972 & 173 & 586125 \\ \hline
\specialcell{ $\forall x_0,x_1\ \pred{sign}(x_1) \wedge \pred{cHas}(x_0, x_1) \rightarrow \pred{signsOn}(x_0)$} & 508 & 119983 & 62 & 496371 \\ \hline
\specialcell{ $\forall x_0,x_1\ \pred{table}(x_1) \wedge \pred{placement}(x_0, x_1) \rightarrow \pred{onTable}(x_0) \vee \pred{leg}(x_0)$} & 11635 & 200110 & 998 & 404181 \\ \hline
\specialcell{ $\forall x_0,x_1\ \pred{table}(x_0) \wedge \pred{cHas}(x_0, x_1) \rightarrow \pred{onTable}(x_1) \vee \pred{leg}(x_1) \vee $ \\ $\pred{shelf}(x_1)$} & 752 & 213507 & 86 & 402579 \\ \hline
\specialcell{ $\forall x_0,x_1\ \pred{hill}(x_1) \wedge \pred{placement}(x_0, x_1) \rightarrow \pred{onHill}(x_0)$} & 1221 & 244159 & 99 & 371445 \\ \hline
\specialcell{ $\forall x_0,x_1\ \pred{placesForHair}(x_1) \wedge \pred{growing on}(x_0, x_1) \rightarrow \pred{hair}(x_0)$} & 10 & 8038 & 0 & 608876 \\ \hline
\specialcell{ $\forall x_0,x_1\ \pred{tree}(x_1) \wedge \pred{growing on}(x_0, x_1) \rightarrow \pred{fruits}(x_0) \vee $ \\ $\pred{branch}(x_0) \vee \pred{leaf}(x_0) \vee \pred{plant}(x_0) \vee \pred{flower}(x_0)$} & 72 & 15764 & 2 & 601086 \\ \hline
\specialcell{ $\forall x_0,x_1\ \pred{wing}(x_1) \wedge \pred{cHas}(x_0, x_1) \rightarrow \pred{bird}(x_0) \vee \pred{planes}(x_0)$} & 774 & 8541 & 28 & 607581 \\ \hline
\specialcell{ $\forall x_0,x_1\ \pred{engine}(x_1) \wedge \pred{related}(x_0, x_1) \wedge  \neg \pred{placement}(x_0, x_1) \rightarrow $ \\ $\pred{transport}(x_0)$} & 411 & 43396 & 43 & 573074 \\ \hline
\specialcell{ $\forall x_0,x_1\ \pred{vase}(x_1) \wedge \pred{in}(x_0, x_1) \rightarrow \pred{inVase}(x_0)$} & 1023 & 8984 & 33 & 606884 \\ \hline
\specialcell{ $\forall x_0,x_1\ \pred{looking at}(x_0, x_1) \rightarrow \pred{human}(x_0) \vee \pred{animals}(x_0) \vee \pred{eye}(x_0)$} & 910 & 169140 & 8 & 446866 \\ \hline
\specialcell{ $\forall x_0,x_1\ \pred{watching}(x_0, x_1) \rightarrow \pred{human}(x_0) \vee \pred{animals}(x_0)$} & 821 & 166534 & 7 & 449562 \\ \hline
\specialcell{ $\forall x_0,x_1\ \pred{covering}(x_0, x_1) \wedge  \neg \pred{human}(x_0) \rightarrow \pred{covers}(x_0)$} & 443 & 116847 & 64 & 499570 \\ \hline
\specialcell{ $\forall x_0,x_1\ \pred{growing on}(x_0, x_1) \rightarrow \pred{grows}(x_0)$} & 176 & 41001 & 5 & 575742 \\ \hline
\specialcell{ $\forall x_0,x_1\ \pred{riding}(x_0, x_1) \rightarrow \pred{human}(x_0)$} & 3009 & 120253 & 77 & 493585 \\ \hline
\specialcell{ $\forall x_0,x_1\ \pred{attached to}(x_0, x_1) \rightarrow \pred{canAttach}(x_0)$} & 1199 & 103684 & 351 & 511690 \\ \hline
\specialcell{ $\forall x_0,x_1\ \pred{walking}(x_0, x_1) \rightarrow \pred{human}(x_0) \vee \pred{animals}(x_0)$} & 1670 & 165685 & 2 & 449567 \\ \hline
\specialcell{ $\forall x_0,x_1\ \pred{parked on}(x_0, x_1) \rightarrow \pred{autos}(x_0) \vee \pred{bikes}(x_0)$} & 753 & 25694 & 8 & 590469 \\ \hline
\specialcell{ $\forall x_0,x_1\ \pred{hold}(x_0, x_1) \rightarrow \pred{canHold}(x_0)$} & 8797 & 142026 & 588 & 465513 \\ \hline
\specialcell{ $\forall x_0,x_1\ \pred{sitting on}(x_0, x_1) \rightarrow \pred{human}(x_0) \vee \pred{animal}(x_0)$} & 2537 & 121606 & 1772 & 491009 \\ \hline
\specialcell{ $\forall x_0,x_1\ \pred{wearingExact}(x_0, x_1) \rightarrow \pred{human}(x_0) \wedge \pred{clothing}(x_1)$} & 39782 & 15649 & 794 & 560699 \\ \hline
\specialcell{ $\forall x_0,x_1\ \pred{house}(x_0) \wedge \pred{window}(x_1) \wedge \pred{related}(x_0, x_1) \rightarrow \pred{cHas}(x_0, x_1)$} & 181 & 64714 & 1 & 552028 \\ \hline
\specialcell{ $\forall x_0,x_1\ \pred{bag}(x_0) \wedge \pred{horse}(x_1) \wedge \pred{related}(x_0, x_1) \rightarrow \pred{on}(x_0, x_1)$} & 3 & 101840 & 0 & 515081 \\ \hline
\specialcell{ $\forall x_0,x_1\ \pred{snow}(x_0) \wedge  \neg \pred{track}(x_1) \wedge  \neg \pred{snow}(x_1) \wedge \pred{related}(x_0, x_1) \rightarrow $ \\ $\pred{placement}(x_0, x_1) \vee \pred{covering}(x_0, x_1)$} & 1395 & 173935 & 57 & 441537 \\ \hline
\specialcell{ $\forall x_0,x_1\ \pred{snow}(x_1) \wedge  \neg \pred{track}(x_0) \wedge  \neg \pred{snow}(x_0) \wedge \pred{related}(x_0, x_1) \rightarrow $ \\ $\pred{covered in}(x_0, x_1) \vee \pred{placement}(x_0, x_1) \vee \pred{has}(x_0, x_1)$} & 3564 & 225581 & 295 & 387484 \\ \hline
\specialcell{ $\forall x_0,x_1\ \pred{surfboard}(x_0) \wedge \pred{wave}(x_1) \wedge \pred{related}(x_0, x_1) \rightarrow $ \\ $\pred{riding}(x_0, x_1) \vee \pred{on}(x_0, x_1) \vee \pred{in}(x_0, x_1) \vee \pred{above}(x_0, x_1)$} & 113 & 129270 & 6 & 487535 \\ \hline
\specialcell{ $\forall x_0,x_1\ \pred{human}(x_0) \wedge \pred{transport}(x_1) \wedge \pred{related}(x_0, x_1) \rightarrow $ \\ $\pred{riding}(x_0, x_1) \vee \pred{placement}(x_0, x_1)$} & 4310 & 172607 & 249 & 439758 \\ \hline

\specialcell{ $\forall x_0,x_1\ \pred{bird}(x_0) \vee \pred{planes}(x_0) \wedge \pred{wing}(x_1) \wedge \pred{related}(x_0, x_1) \rightarrow $ \\ $\pred{cHas}(x_0, x_1)$} & 774 & 64121 & 4 & 552025 \\ \hline
\end{tabular}
\caption{The second set of rules for the Visual Genome dataset.}
\label{table:vs_rules2}
\end{table}
\begin{table}[]
\begin{tabular}{l|l|l|l|l}
\hline
Formula & $a, c$ & $\neg a, c$ & $a, \neg c$ & $\neg a, \neg c$ \\ \hline
\specialcell{ $\forall x_0,x_1\ \pred{finger}(x_0) \wedge \pred{hand}(x_1) \wedge \pred{related}(x_0, x_1) \rightarrow $ \\ $\pred{attached to}(x_0, x_1) \vee \pred{on}(x_0, x_1) \vee \pred{of}(x_0, x_1)$} & 208 & 129215 & 9 & 487492 \\ \hline
\specialcell{ $\forall x_0,x_1\ \pred{sign}(x_0) \wedge \pred{signsOn}(x_1) \wedge \pred{related}(x_0, x_1) \rightarrow $ \\ $\pred{connected}(x_0, x_1) \vee \pred{placement}(x_0, x_1)$} & 5205 & 171914 & 138 & 439667 \\ \hline
\specialcell{ $\forall x_0,x_1\ \pred{basket}(x_0) \wedge \pred{basketOn}(x_1) \wedge \pred{related}(x_0, x_1) \rightarrow $ \\ $\pred{placement}(x_0, x_1) \vee \pred{connected}(x_0, x_1)$} & 345 & 176774 & 3 & 439802 \\ \hline
\specialcell{ $\forall x_0,x_1\ \pred{head}(x_0) \wedge \pred{headHas}(x_1) \wedge \pred{related}(x_0, x_1) \rightarrow \pred{cHas}(x_0, x_1) \vee $ \\ $\pred{on}(x_0, x_1)$} & 298 & 166134 & 25 & 450467 \\ \hline
\specialcell{ $\forall x_0,x_1\ \pred{autos}(x_0) \wedge \pred{autosHas}(x_1) \wedge \pred{related}(x_0, x_1) \rightarrow $ \\ $\pred{cHas}(x_0, x_1)$} & 2184 & 62711 & 153 & 551876 \\ \hline
\specialcell{ $\forall x_0,x_1\ \pred{planes}(x_0) \wedge \pred{planesHas}(x_1) \wedge \pred{related}(x_0, x_1) \rightarrow $ \\ $\pred{cHas}(x_0, x_1)$} & 1796 & 63099 & 18 & 552011 \\ \hline
\specialcell{ $\forall x_0,x_1\ \pred{glass}(x_0) \wedge \pred{glassOn}(x_1) \wedge \pred{related}(x_0, x_1) \rightarrow $ \\ $\pred{placement}(x_0, x_1)$} & 2609 & 172287 & 58 & 441970 \\ \hline
\specialcell{ $\forall x_0,x_1\ \pred{tree}(x_0) \wedge \pred{treeOn}(x_1) \wedge \pred{related}(x_0, x_1) \rightarrow $ \\ $\pred{placement}(x_0, x_1)$} & 3530 & 171366 & 321 & 441707 \\ \hline
\specialcell{ $\forall x_0,x_1\ \pred{curtain}(x_0) \wedge \pred{curtainOn}(x_1) \wedge \pred{related}(x_0, x_1) \rightarrow $ \\ $\pred{placement}(x_0, x_1) \vee \pred{covering}(x_0, x_1) \vee \pred{hanging from}(x_0, x_1)$} & 738 & 175271 & 8 & 440907 \\ \hline
\specialcell{ $\forall x_0,x_1\ \pred{arm}(x_1) \wedge \pred{hasArm}(x_0) \wedge \pred{related}(x_0, x_1) \rightarrow \pred{cHas}(x_0, x_1)$} & 1852 & 63043 & 30 & 551999 \\ \hline
\specialcell{ $\forall x_0,x_1\ \pred{tail}(x_1) \wedge \pred{hasTail}(x_0) \wedge \pred{related}(x_0, x_1) \rightarrow \pred{cHas}(x_0, x_1)$} & 2380 & 62515 & 18 & 552011 \\ \hline
\specialcell{ $\forall x_0,x_1\ \pred{leg}(x_1) \wedge \pred{hasLeg}(x_0) \wedge \pred{related}(x_0, x_1) \rightarrow \pred{cHas}(x_0, x_1)$} & 4803 & 60092 & 137 & 551892 \\ \hline
\specialcell{ $\forall x_0,x_1\ \pred{face}(x_1) \wedge \pred{hasFace}(x_0) \wedge \pred{related}(x_0, x_1) \rightarrow \pred{cHas}(x_0, x_1)$} & 1701 & 63194 & 28 & 552001 \\ \hline
\specialcell{ $\forall x_0,x_1\ \pred{human}(x_1) \wedge \pred{onHuman}(x_0) \wedge \pred{related}(x_0, x_1) \rightarrow \pred{on}(x_0, x_1) \vee $ \\ $\pred{of}(x_0, x_1)$} & 17752 & 110322 & 869 & 487981 \\ \hline
\specialcell{ $\forall x_0,x_1\ \pred{window}(x_1) \wedge \pred{hasWindow}(x_0) \wedge \pred{related}(x_0, x_1) \rightarrow $ \\ $\pred{cHas}(x_0, x_1)$} & 3299 & 61596 & 114 & 551915 \\ \hline
\specialcell{ $\forall x_0,x_1\ \pred{pole}(x_1) \wedge \pred{onPole}(x_0) \wedge \pred{related}(x_0, x_1) \rightarrow \pred{on}(x_0, x_1) \vee $ \\ $\pred{connected}(x_0, x_1)$} & 3086 & 101062 & 245 & 512531 \\ \hline
\specialcell{ $\forall x_0,x_1\ \pred{sign}(x_1) \wedge \pred{signsOn}(x_0) \wedge \pred{related}(x_0, x_1) \rightarrow \pred{cHas}(x_0, x_1)$} & 508 & 64387 & 791 & 551238 \\ \hline
\specialcell{ $\forall x_0,x_1\ \pred{table}(x_1) \wedge \pred{onTable}(x_0) \wedge \pred{related}(x_0, x_1) \rightarrow $ \\ $\pred{placement}(x_0, x_1)$} & 11539 & 163357 & 62 & 441966 \\ \hline
\specialcell{ $\forall x_0,x_1\ \pred{hill}(x_1) \wedge \pred{onHill}(x_0) \wedge \pred{related}(x_0, x_1) \rightarrow $ \\ $\pred{placement}(x_0, x_1)$} & 1221 & 173675 & 54 & 441974 \\ \hline
\specialcell{ $\forall x_0,x_1\ \pred{streets}(x_1) \wedge \pred{onStreet}(x_0) \wedge \pred{related}(x_0, x_1) \rightarrow $ \\ $\pred{placement}(x_0, x_1) \vee \pred{parked on}(x_0, x_1) \vee \pred{walking}(x_0, x_1)$} & 10645 & 166326 & 81 & 439872 \\ \hline
\specialcell{ $\forall x_0,x_1\ \pred{autos}(x_1) \wedge \pred{autosHas}(x_0) \wedge \pred{related}(x_0, x_1) \rightarrow $ \\ $\pred{placement}(x_0, x_1) \vee \pred{of}(x_0, x_1)$} & 7336 & 193638 & 281 & 415669 \\ \hline
\specialcell{ $\forall x_0,x_1\ \pred{vase}(x_1) \wedge \pred{inVase}(x_0) \wedge \pred{related}(x_0, x_1) \rightarrow \pred{in}(x_0, x_1) \vee $ \\ $\pred{on}(x_0, x_1)$} & 1067 & 119976 & 48 & 495833 \\ \hline
\specialcell{ $\forall x_0,x_1\ \pred{clothing}(x_0) \wedge \pred{related}(x_0, x_1) \rightarrow \pred{of}(x_0, x_1) \vee $ \\ $\pred{cHas}(x_0, x_1) \vee \pred{placement}(x_0, x_1)$} & 17241 & 247665 & 496 & 351522 \\ \hline
\specialcell{ $\forall x_0,x_1\ \pred{arm}(x_0) \wedge \pred{related}(x_0, x_1) \rightarrow \pred{on}(x_0, x_1) \vee \pred{of}(x_0, x_1)$} & 1455 & 126619 & 254 & 488596 \\ \hline
\specialcell{ $\forall x_0,x_1\ \pred{cat}(x_0) \wedge \pred{related}(x_0, x_1) \rightarrow \pred{on}(x_0, x_1) \vee \pred{cHas}(x_0, x_1) \vee $ \\ $\pred{relationsOn}(x_0, x_1) \vee \pred{in}(x_0, x_1)$} & 3257 & 187810 & 392 & 425465 \\ \hline
\specialcell{ $\forall x_0,x_1\ \pred{engine}(x_0) \wedge \pred{related}(x_0, x_1) \rightarrow \pred{engineO}(x_0, x_1)$} & 1005 & 201261 & 71 & 414587 \\ \hline
\specialcell{ $\forall x_0,x_1\ \pred{shirt}(x_1) \wedge \pred{related}(x_0, x_1) \rightarrow \pred{wearingAll}(x_0, x_1)$} & 15092 & 207441 & 117 & 394274 \\ \hline
\specialcell{ $\forall x_0,x_1\ \pred{clothing}(x_1) \wedge \pred{related}(x_0, x_1) \wedge  \neg \pred{bag}(x_1) \rightarrow $ \\ $\pred{wearingAll}(x_0, x_1)$} & 51374 & 171159 & 1632 & 392759 \\ \hline
\specialcell{ $\forall x_0,x_1\ \pred{bag}(x_1) \wedge \pred{related}(x_0, x_1) \rightarrow \pred{wearingAll}(x_0, x_1) \vee $ \\ $\pred{holding}(x_0, x_1) \vee \pred{carrying}(x_0, x_1)$} & 1424 & 229369 & 146 & 385985 \\ \hline
\specialcell{ $\forall x_0,x_1\ \pred{bodypartAll}(x_1) \wedge  \neg \pred{specialBodyparts}(x_1) \wedge $ \\ $\pred{related}(x_0, x_1) \rightarrow \pred{cHas}(x_0, x_1) \vee \pred{placement}(x_0, x_1)$} & 26611 & 212303 & 483 & 377527 \\ \hline
\specialcell{ $\forall x_0,x_1\ \pred{umbrella}(x_1) \wedge \pred{related}(x_0, x_1) \rightarrow \pred{umbrellaS}(x_0, x_1)$} & 1938 & 103457 & 344 & 511185 \\ \hline
\specialcell{ $\forall x_0,x_1\ \pred{relationsOn}(x_0, x_1) \rightarrow \pred{on}(x_0, x_1)$} & 1358 & 100485 & 5984 & 509097 \\ \hline
\specialcell{ $\forall x_0,x_1,x_2\ \pred{hair}(x_1) \wedge \pred{ear}(x_2) \wedge \pred{in}(x_1, x_2) \wedge \pred{cHas}(x_0, x_2) \rightarrow $ \\ $\pred{animals}(x_0)$} & 5 & 305776 & 0 & 3969033 \\ \hline
\end{tabular}
\caption{The third set of rules for the Visual Genome dataset.}
\label{table:vs_rules3}
\end{table}

\begin{table}[]
\begin{tabular}{l|l|l}
    \hline 
Category name & Arity & Options \\ \hline
$\pred{animals}$ & 1 & \specialcell{$\pred{animal}$, $\pred{bear}$, $\pred{bird}$, $\pred{cat}$, $\pred{cow}$, $\pred{dog}$, $\pred{elephant}$, $\pred{giraffe}$, $\pred{horse}$,  \\ $\pred{sheep}$, $\pred{zebra}$} \\ \hline
$\pred{autos}$ & 1 & \specialcell{$\pred{bus}$, $\pred{car}$, $\pred{truck}$, $\pred{vehicle}$} \\ \hline
$\pred{autosHas}$ & 1 & \specialcell{$\pred{door}$, $\pred{engine}$, $\pred{handle}$, $\pred{light}$, $\pred{logo}$, $\pred{plate}$, $\pred{roof}$, $\pred{seat}$, $\pred{sign}$, $\pred{tire}$,  \\ $\pred{trunk}$, $\pred{wheel}$, $\pred{window}$, $\pred{windshield}$} \\ \hline
$\pred{basketOn}$ & 1 & \specialcell{$\pred{bike}$, $\pred{counter}$, $\pred{desk}$, $\pred{motorcycle}$, $\pred{pole}$, $\pred{shelf}$, $\pred{table}$, $\pred{toilet}$} \\ \hline
$\pred{bikes}$ & 1 & \specialcell{$\pred{bike}$, $\pred{motorcycle}$} \\ \hline
$\pred{bodypart}$ & 1 & \specialcell{$\pred{ear}$, $\pred{eye}$, $\pred{face}$, $\pred{hair}$, $\pred{head}$, $\pred{leg}$, $\pred{mouth}$, $\pred{neck}$, $\pred{nose}$} \\ \hline
$\pred{bodypartAll}$ & 1 & \specialcell{$\pred{arm}$, $\pred{ear}$, $\pred{eye}$, $\pred{face}$, $\pred{finger}$, $\pred{hair}$, $\pred{hand}$, $\pred{head}$, $\pred{leg}$, $\pred{mouth}$, $\pred{neck}$,  \\ $\pred{nose}$, $\pred{paw}$, $\pred{tail}$} \\ \hline
$\pred{bodypartAnimal}$ & 1 & \specialcell{$\pred{paw}$, $\pred{tail}$} \\ \hline
$\pred{bodypartHuman}$ & 1 & \specialcell{$\pred{arm}$, $\pred{finger}$, $\pred{hand}$} \\ \hline
$\pred{cHas}$ & 2 & \specialcell{$\pred{has}$, $\pred{with}$} \\ \hline
$\pred{canAttach}$ & 1 & \specialcell{$\pred{boot}$, $\pred{branch}$, $\pred{clock}$, $\pred{door}$, $\pred{engine}$, $\pred{finger}$, $\pred{flag}$, $\pred{hand}$, $\pred{handle}$,  \\ $\pred{leaf}$, $\pred{leg}$, $\pred{letter}$, $\pred{light}$, $\pred{pole}$, $\pred{sign}$, $\pred{tail}$, $\pred{tire}$, $\pred{tower}$, $\pred{trunk}$,  \\ $\pred{wheel}$, $\pred{window}$, $\pred{windshield}$, $\pred{wing}$, $\pred{wire}$} \\ \hline
$\pred{canAttachTo}$ & 1 & \specialcell{$\pred{airplane}$, $\pred{bag}$, $\pred{bike}$, $\pred{boat}$, $\pred{boy}$, $\pred{branch}$, $\pred{building}$, $\pred{bus}$, $\pred{car}$, $\pred{child}$,  \\ $\pred{clock}$, $\pred{cup}$, $\pred{fence}$, $\pred{flower}$, $\pred{girl}$, $\pred{guy}$, $\pred{hand}$, $\pred{house}$, $\pred{kid}$, $\pred{lady}$,  \\ $\pred{man}$, $\pred{men}$, $\pred{motorcycle}$, $\pred{people}$, $\pred{person}$, $\pred{plane}$, $\pred{player}$, $\pred{pole}$, $\pred{post}$,  \\ $\pred{sign}$, $\pred{ski}$, $\pred{skier}$, $\pred{tower}$, $\pred{train}$, $\pred{tree}$, $\pred{truck}$, $\pred{vehicle}$, $\pred{wing}$, $\pred{woman}$} \\ \hline
$\pred{canHold}$ & 1 & \specialcell{$\pred{boy}$, $\pred{child}$, $\pred{girl}$, $\pred{guy}$, $\pred{hand}$, $\pred{kid}$, $\pred{lady}$, $\pred{man}$, $\pred{men}$, $\pred{people}$, $\pred{person}$,  \\ $\pred{plate}$, $\pred{player}$, $\pred{pole}$, $\pred{post}$, $\pred{shelf}$, $\pred{skier}$, $\pred{vase}$, $\pred{woman}$} \\ \hline
$\pred{clothing}$ & 1 & \specialcell{$\pred{bag}$, $\pred{boot}$, $\pred{cap}$, $\pred{coat}$, $\pred{glass}$, $\pred{glove}$, $\pred{hat}$, $\pred{helmet}$, $\pred{jacket}$, $\pred{jean}$,  \\ $\pred{pant}$, $\pred{shirt}$, $\pred{shoe}$, $\pred{short}$, $\pred{ski}$, $\pred{sneaker}$, $\pred{sock}$, $\pred{tie}$, $\pred{trunk}$} \\ \hline
$\pred{connected}$ & 2 & \specialcell{$\pred{attached to}$, $\pred{hanging from}$, $\pred{mounted on}$} \\ \hline
$\pred{container}$ & 1 & \specialcell{$\pred{basket}$, $\pred{bottle}$, $\pred{bowl}$, $\pred{box}$, $\pred{cup}$, $\pred{glass}$, $\pred{plate}$, $\pred{pot}$, $\pred{vase}$} \\ \hline
$\pred{cover}$ & 2 & \specialcell{$\pred{covered in}$, $\pred{covering}$} \\ \hline
$\pred{covers}$ & 1 & \specialcell{$\pred{bag}$, $\pred{boot}$, $\pred{cap}$, $\pred{coat}$, $\pred{curtain}$, $\pred{glass}$, $\pred{glove}$, $\pred{hair}$, $\pred{hand}$, $\pred{hat}$,  \\ $\pred{helmet}$, $\pred{jacket}$, $\pred{jean}$, $\pred{pant}$, $\pred{rock}$, $\pred{roof}$, $\pred{shirt}$, $\pred{shoe}$, $\pred{short}$, $\pred{ski}$,  \\ $\pred{sneaker}$, $\pred{snow}$, $\pred{sock}$, $\pred{tie}$, $\pred{tree}$, $\pred{trunk}$, $\pred{umbrella}$} \\ \hline
$\pred{curtainOn}$ & 1 & \specialcell{$\pred{bed}$, $\pred{door}$, $\pred{window}$} \\ \hline
$\pred{engineO}$ & 2 & \specialcell{$\pred{above}$, $\pred{across}$, $\pred{against}$, $\pred{along}$, $\pred{at}$, $\pred{attached to}$, $\pred{behind}$, $\pred{between}$,  \\ $\pred{in}$, $\pred{in front of}$, $\pred{laying on}$, $\pred{lying on}$, $\pred{near}$, $\pred{of}$, $\pred{on}$, $\pred{over}$, $\pred{sitting on}$,  \\ $\pred{standing on}$, $\pred{under}$} \\ \hline
$\pred{flora}$ & 1 & \specialcell{$\pred{branch}$, $\pred{flower}$, $\pred{leaf}$, $\pred{plant}$, $\pred{tree}$} \\ \hline
$\pred{fruits}$ & 1 & \specialcell{$\pred{banana}$, $\pred{fruit}$, $\pred{orange}$} \\ \hline
$\pred{furniture}$ & 1 & \specialcell{$\pred{bed}$, $\pred{bench}$, $\pred{cabinet}$, $\pred{chair}$, $\pred{clock}$, $\pred{counter}$, $\pred{desk}$, $\pred{lamp}$, $\pred{sink}$,  \\ $\pred{table}$} \\ \hline
$\pred{glassOn}$ & 1 & \specialcell{$\pred{boy}$, $\pred{building}$, $\pred{child}$, $\pred{counter}$, $\pred{desk}$, $\pred{door}$, $\pred{face}$, $\pred{girl}$, $\pred{guy}$, $\pred{head}$,  \\ $\pred{house}$, $\pred{kid}$, $\pred{lady}$, $\pred{man}$, $\pred{men}$, $\pred{people}$, $\pred{person}$, $\pred{plate}$, $\pred{player}$, $\pred{shelf}$,  \\ $\pred{sink}$, $\pred{skier}$, $\pred{table}$, $\pred{tower}$, $\pred{window}$, $\pred{woman}$} \\ \hline
$\pred{grows}$ & 1 & \specialcell{$\pred{banana}$, $\pred{branch}$, $\pred{flower}$, $\pred{fruit}$, $\pred{hair}$, $\pred{leaf}$, $\pred{orange}$, $\pred{plant}$, $\pred{tree}$} \\ \hline
$\pred{hasArm}$ & 1 & \specialcell{$\pred{bear}$, $\pred{bench}$, $\pred{boy}$, $\pred{chair}$, $\pred{child}$, $\pred{clock}$, $\pred{girl}$, $\pred{guy}$, $\pred{kid}$, $\pred{lady}$,  \\ $\pred{man}$, $\pred{men}$, $\pred{people}$, $\pred{person}$, $\pred{player}$, $\pred{skier}$, $\pred{woman}$} \\ \hline
$\pred{hasFace}$ & 1 & \specialcell{$\pred{animal}$, $\pred{bear}$, $\pred{bird}$, $\pred{boy}$, $\pred{cat}$, $\pred{child}$, $\pred{clock}$, $\pred{cow}$, $\pred{dog}$, $\pred{elephant}$,  \\ $\pred{giraffe}$, $\pred{girl}$, $\pred{guy}$, $\pred{head}$, $\pred{horse}$, $\pred{kid}$, $\pred{lady}$, $\pred{man}$, $\pred{men}$, $\pred{people}$,  \\ $\pred{person}$, $\pred{player}$, $\pred{sheep}$, $\pred{skier}$, $\pred{train}$, $\pred{woman}$, $\pred{zebra}$} \\ \hline
$\pred{hasLeg}$ & 1 & \specialcell{$\pred{animal}$, $\pred{bear}$, $\pred{bench}$, $\pred{bird}$, $\pred{boy}$, $\pred{cat}$, $\pred{chair}$, $\pred{child}$, $\pred{cow}$, $\pred{desk}$,  \\ $\pred{dog}$, $\pred{elephant}$, $\pred{giraffe}$, $\pred{girl}$, $\pred{guy}$, $\pred{horse}$, $\pred{kid}$, $\pred{lady}$, $\pred{man}$, $\pred{men}$,  \\ $\pred{pant}$, $\pred{people}$, $\pred{person}$, $\pred{player}$, $\pred{sheep}$, $\pred{skier}$, $\pred{table}$, $\pred{woman}$, $\pred{zebra}$} \\ \hline
$\pred{hasTail}$ & 1 & \specialcell{$\pred{airplane}$, $\pred{animal}$, $\pred{bear}$, $\pred{bird}$, $\pred{cat}$, $\pred{cow}$, $\pred{dog}$, $\pred{elephant}$, $\pred{giraffe}$,  \\ $\pred{horse}$, $\pred{kite}$, $\pred{plane}$, $\pred{sheep}$, $\pred{zebra}$} \\ \hline
$\pred{hasWindow}$ & 1 & \specialcell{$\pred{airplane}$, $\pred{boat}$, $\pred{building}$, $\pred{bus}$, $\pred{car}$, $\pred{door}$, $\pred{house}$, $\pred{plane}$, $\pred{roof}$,  \\ $\pred{tower}$, $\pred{train}$, $\pred{truck}$, $\pred{vehicle}$} \\ \hline
\end{tabular}
\caption{The first set of category definitions for the Visual Genome ontology.}
\label{table:categories1}
\end{table}

\begin{table}[]
    \begin{tabular}{l|l|l}
    \hline 
Category name & Arity & Options \\ \hline
$\pred{headHas}$ & 1 & \specialcell{$\pred{cap}$, $\pred{ear}$, $\pred{eye}$, $\pred{face}$, $\pred{hair}$, $\pred{hat}$, $\pred{helmet}$, $\pred{mouth}$, $\pred{nose}$} \\ \hline
$\pred{headwear}$ & 1 & \specialcell{$\pred{cap}$, $\pred{hat}$, $\pred{helmet}$} \\ \hline
$\pred{hold}$ & 2 & \specialcell{$\pred{carrying}$, $\pred{holding}$} \\ \hline
$\pred{human}$ & 1 & \specialcell{$\pred{boy}$, $\pred{child}$, $\pred{girl}$, $\pred{guy}$, $\pred{kid}$, $\pred{lady}$, $\pred{man}$, $\pred{men}$, $\pred{people}$, $\pred{person}$, $\pred{player}$,  \\ $\pred{skier}$, $\pred{woman}$} \\ \hline
$\pred{inVase}$ & 1 & \specialcell{$\pred{flower}$, $\pred{leaf}$, $\pred{plant}$} \\ \hline
$\pred{kitchenware}$ & 1 & \specialcell{$\pred{banana}$, $\pred{basket}$, $\pred{bottle}$, $\pred{bowl}$, $\pred{box}$, $\pred{cup}$, $\pred{flower}$, $\pred{food}$, $\pred{fork}$, $\pred{fruit}$,  \\ $\pred{glass}$, $\pred{orange}$, $\pred{pizza}$, $\pred{plant}$, $\pred{plate}$, $\pred{pot}$, $\pred{towel}$, $\pred{vase}$, $\pred{vegetable}$} \\ \hline
$\pred{office}$ & 1 & \specialcell{$\pred{book}$, $\pred{clock}$, $\pred{laptop}$, $\pred{light}$, $\pred{paper}$, $\pred{phone}$, $\pred{screen}$} \\ \hline
$\pred{onHill}$ & 1 & \specialcell{$\pred{animal}$, $\pred{bear}$, $\pred{bench}$, $\pred{bird}$, $\pred{boy}$, $\pred{building}$, $\pred{cat}$, $\pred{child}$, $\pred{cow}$, $\pred{dog}$,  \\ $\pred{elephant}$, $\pred{fence}$, $\pred{giraffe}$, $\pred{girl}$, $\pred{guy}$, $\pred{horse}$, $\pred{house}$, $\pred{kid}$, $\pred{lady}$,  \\ $\pred{man}$, $\pred{men}$, $\pred{people}$, $\pred{person}$, $\pred{plant}$, $\pred{player}$, $\pred{pole}$, $\pred{rock}$, $\pred{sheep}$, $\pred{sign}$,  \\ $\pred{skier}$, $\pred{snow}$, $\pred{tower}$, $\pred{tree}$, $\pred{woman}$, $\pred{zebra}$} \\ \hline
$\pred{onHuman}$ & 1 & \specialcell{$\pred{arm}$, $\pred{bag}$, $\pred{boot}$, $\pred{cap}$, $\pred{coat}$, $\pred{ear}$, $\pred{eye}$, $\pred{face}$, $\pred{finger}$, $\pred{glass}$, $\pred{glove}$,  \\ $\pred{hair}$, $\pred{hand}$, $\pred{hat}$, $\pred{head}$, $\pred{helmet}$, $\pred{jacket}$, $\pred{jean}$, $\pred{leg}$, $\pred{mouth}$, $\pred{neck}$,  \\ $\pred{nose}$, $\pred{pant}$, $\pred{shirt}$, $\pred{shoe}$, $\pred{short}$, $\pred{ski}$, $\pred{sneaker}$, $\pred{sock}$, $\pred{tie}$, $\pred{trunk}$} \\ \hline
$\pred{onPole}$ & 1 & \specialcell{$\pred{bird}$, $\pred{box}$, $\pred{clock}$, $\pred{flag}$, $\pred{handle}$, $\pred{lamp}$, $\pred{light}$, $\pred{sign}$, $\pred{umbrella}$,  \\ $\pred{wire}$} \\ \hline
$\pred{onStreet}$ & 1 & \specialcell{$\pred{bag}$, $\pred{bench}$, $\pred{bike}$, $\pred{boy}$, $\pred{bus}$, $\pred{car}$, $\pred{chair}$, $\pred{child}$, $\pred{dog}$, $\pred{fence}$, $\pred{girl}$,  \\ $\pred{guy}$, $\pred{kid}$, $\pred{lady}$, $\pred{light}$, $\pred{man}$, $\pred{men}$, $\pred{motorcycle}$, $\pred{people}$, $\pred{person}$,  \\ $\pred{player}$, $\pred{pole}$, $\pred{post}$, $\pred{sign}$, $\pred{skateboard}$, $\pred{skier}$, $\pred{snow}$, $\pred{tile}$, $\pred{tree}$,  \\ $\pred{truck}$, $\pred{vehicle}$, $\pred{woman}$} \\ \hline
$\pred{onTable}$ & 1 & \specialcell{$\pred{bag}$, $\pred{banana}$, $\pred{basket}$, $\pred{book}$, $\pred{bottle}$, $\pred{bowl}$, $\pred{box}$, $\pred{boy}$, $\pred{cat}$, $\pred{chair}$,  \\ $\pred{child}$, $\pred{clock}$, $\pred{cup}$, $\pred{flower}$, $\pred{food}$, $\pred{fork}$, $\pred{fruit}$, $\pred{girl}$, $\pred{glass}$, $\pred{guy}$,  \\ $\pred{hand}$, $\pred{kid}$, $\pred{lady}$, $\pred{lamp}$, $\pred{laptop}$, $\pred{light}$, $\pred{man}$, $\pred{men}$, $\pred{orange}$, $\pred{paper}$,  \\ $\pred{people}$, $\pred{person}$, $\pred{phone}$, $\pred{pizza}$, $\pred{plant}$, $\pred{plate}$, $\pred{player}$, $\pred{pot}$, $\pred{screen}$,  \\ $\pred{skier}$, $\pred{towel}$, $\pred{vase}$, $\pred{vegetable}$, $\pred{woman}$} \\ \hline
$\pred{otherTransport}$ & 1 & \specialcell{$\pred{bike}$, $\pred{boat}$, $\pred{motorcycle}$, $\pred{train}$} \\ \hline
$\pred{outsideNature}$ & 1 & \specialcell{$\pred{beach}$, $\pred{branch}$, $\pred{flower}$, $\pred{hill}$, $\pred{mountain}$, $\pred{rock}$, $\pred{tree}$} \\ \hline
$\pred{outsidePlaces}$ & 1 & \specialcell{$\pred{beach}$, $\pred{hill}$, $\pred{mountain}$, $\pred{sidewalk}$, $\pred{street}$, $\pred{track}$} \\ \hline
$\pred{outsidePlacesCity}$ & 1 & \specialcell{$\pred{sidewalk}$, $\pred{street}$, $\pred{track}$} \\ \hline
$\pred{outsidePlacesNature}$ & 1 & \specialcell{$\pred{beach}$, $\pred{hill}$, $\pred{mountain}$} \\ \hline
$\pred{outsideStationary}$ & 1 & \specialcell{$\pred{airplane}$, $\pred{beach}$, $\pred{bench}$, $\pred{bike}$, $\pred{boat}$, $\pred{branch}$, $\pred{building}$, $\pred{bus}$, $\pred{car}$,  \\ $\pred{flower}$, $\pred{hill}$, $\pred{house}$, $\pred{motorcycle}$, $\pred{mountain}$, $\pred{plane}$, $\pred{rock}$, $\pred{roof}$,  \\ $\pred{sidewalk}$, $\pred{snow}$, $\pred{street}$, $\pred{tower}$, $\pred{track}$, $\pred{train}$, $\pred{tree}$, $\pred{truck}$, $\pred{vehicle}$} \\ \hline
$\pred{placement}$ & 2 & \specialcell{$\pred{above}$, $\pred{across}$, $\pred{against}$, $\pred{along}$, $\pred{at}$, $\pred{behind}$, $\pred{between}$, $\pred{in}$, $\pred{in front of}$,  \\ $\pred{laying on}$, $\pred{lying on}$, $\pred{near}$, $\pred{on}$, $\pred{over}$, $\pred{sitting on}$, $\pred{standing on}$,  \\ $\pred{under}$} \\ \hline
$\pred{placesForHair}$ & 1 & \specialcell{$\pred{arm}$, $\pred{cat}$, $\pred{dog}$, $\pred{head}$, $\pred{horse}$, $\pred{leg}$, $\pred{neck}$, $\pred{tail}$} \\ \hline
$\pred{placesToWalkOn}$ & 1 & \specialcell{$\pred{beach}$, $\pred{hill}$, $\pred{mountain}$, $\pred{rock}$, $\pred{sidewalk}$, $\pred{snow}$, $\pred{street}$} \\ \hline
$\pred{planes}$ & 1 & \specialcell{$\pred{airplane}$, $\pred{plane}$} \\ \hline
$\pred{planesHas}$ & 1 & \specialcell{$\pred{door}$, $\pred{engine}$, $\pred{light}$, $\pred{logo}$, $\pred{nose}$, $\pred{number}$, $\pred{seat}$, $\pred{tail}$, $\pred{tire}$, $\pred{wheel}$,  \\ $\pred{window}$, $\pred{windshield}$, $\pred{wing}$} \\ \hline
$\pred{professions}$ & 1 & \specialcell{$\pred{player}$, $\pred{skier}$} \\ \hline
$\pred{relationsOn}$ & 2 & \specialcell{$\pred{laying on}$, $\pred{lying on}$, $\pred{sitting on}$, $\pred{standing on}$} \\ \hline
$\pred{ridingOn}$ & 1 & \specialcell{$\pred{airplane}$, $\pred{bike}$, $\pred{board}$, $\pred{boat}$, $\pred{bus}$, $\pred{car}$, $\pred{elephant}$, $\pred{horse}$, $\pred{motorcycle}$,  \\ $\pred{plane}$, $\pred{skateboard}$, $\pred{ski}$, $\pred{surfboard}$, $\pred{train}$, $\pred{truck}$, $\pred{vehicle}$, $\pred{wave}$} \\ \hline
$\pred{semanticR}$ & 2 & \specialcell{$\pred{carrying}$, $\pred{covered in}$, $\pred{covering}$, $\pred{growing on}$, $\pred{holding}$, $\pred{laying on}$,  \\ $\pred{looking at}$, $\pred{lying on}$, $\pred{on back of}$, $\pred{parked on}$, $\pred{riding}$, $\pred{sitting on}$,  \\ $\pred{standing on}$, $\pred{walking on}$, $\pred{watching}$, $\pred{wearing}$, $\pred{wears}$} \\ \hline
$\pred{signsOn}$ & 1 & \specialcell{$\pred{boat}$, $\pred{building}$, $\pred{bus}$, $\pred{car}$, $\pred{door}$, $\pred{fence}$, $\pred{pole}$, $\pred{post}$, $\pred{sidewalk}$,  \\ $\pred{street}$, $\pred{train}$, $\pred{tree}$, $\pred{truck}$, $\pred{window}$} \\ \hline
\end{tabular}
\caption{The second set of category definitions for the Visual Genome ontology.}
\label{table:categories2}
\end{table}

\begin{table}[]
    \begin{tabular}{l|l|l}
    \hline 
Category name & Arity & Options \\ \hline
$\pred{specialBodyparts}$ & 1 & \specialcell{$\pred{arm}$, $\pred{face}$, $\pred{leg}$, $\pred{tail}$} \\ \hline
$\pred{sport}$ & 1 & \specialcell{$\pred{kite}$, $\pred{racket}$, $\pred{skateboard}$, $\pred{surfboard}$} \\ \hline
$\pred{streets}$ & 1 & \specialcell{$\pred{sidewalk}$, $\pred{street}$} \\ \hline
$\pred{structure}$ & 1 & \specialcell{$\pred{building}$, $\pred{house}$, $\pred{tower}$} \\ \hline
$\pred{structureHas}$ & 1 & \specialcell{$\pred{clock}$, $\pred{door}$, $\pred{fence}$, $\pred{flag}$, $\pred{light}$, $\pred{pole}$, $\pred{roof}$, $\pred{sign}$, $\pred{tower}$, $\pred{window}$} \\ \hline
$\pred{thingsIn}$ & 1 & \specialcell{$\pred{airplane}$, $\pred{bag}$, $\pred{basket}$, $\pred{beach}$, $\pred{bed}$, $\pred{bike}$, $\pred{boat}$, $\pred{boot}$, $\pred{bottle}$,  \\ $\pred{bowl}$, $\pred{box}$, $\pred{building}$, $\pred{bus}$, $\pred{cap}$, $\pred{car}$, $\pred{chair}$, $\pred{coat}$, $\pred{counter}$, $\pred{cup}$,  \\ $\pred{fence}$, $\pred{glass}$, $\pred{glove}$, $\pred{hand}$, $\pred{hat}$, $\pred{helmet}$, $\pred{house}$, $\pred{jacket}$, $\pred{jean}$,  \\ $\pred{motorcycle}$, $\pred{pant}$, $\pred{plane}$, $\pred{plate}$, $\pred{pot}$, $\pred{shirt}$, $\pred{shoe}$, $\pred{short}$, $\pred{ski}$,  \\ $\pred{sneaker}$, $\pred{snow}$, $\pred{sock}$, $\pred{stand}$, $\pred{street}$, $\pred{tie}$, $\pred{tower}$, $\pred{train}$, $\pred{tree}$,  \\ $\pred{truck}$, $\pred{trunk}$, $\pred{vase}$, $\pred{vehicle}$, $\pred{wave}$, $\pred{window}$} \\ \hline
$\pred{thingsOn}$ & 1 & \specialcell{$\pred{bed}$, $\pred{bench}$, $\pred{building}$, $\pred{cabinet}$, $\pred{chair}$, $\pred{clock}$, $\pred{counter}$, $\pred{desk}$, $\pred{house}$,  \\ $\pred{lamp}$, $\pred{laptop}$, $\pred{sink}$, $\pred{street}$, $\pred{table}$, $\pred{toilet}$, $\pred{tower}$} \\ \hline
$\pred{thingsToHold}$ & 1 & \specialcell{$\pred{animal}$, $\pred{bag}$, $\pred{banana}$, $\pred{basket}$, $\pred{bear}$, $\pred{bike}$, $\pred{bird}$, $\pred{board}$, $\pred{book}$, $\pred{boot}$,  \\ $\pred{bottle}$, $\pred{bowl}$, $\pred{box}$, $\pred{boy}$, $\pred{cap}$, $\pred{cat}$, $\pred{child}$, $\pred{clock}$, $\pred{coat}$, $\pred{cow}$, $\pred{cup}$,  \\ $\pred{dog}$, $\pred{elephant}$, $\pred{flag}$, $\pred{flower}$, $\pred{food}$, $\pred{fork}$, $\pred{fruit}$, $\pred{giraffe}$, $\pred{girl}$,  \\ $\pred{glass}$, $\pred{glove}$, $\pred{hand}$, $\pred{handle}$, $\pred{hat}$, $\pred{helmet}$, $\pred{horse}$, $\pred{jacket}$, $\pred{jean}$,  \\ $\pred{kite}$, $\pred{laptop}$, $\pred{light}$, $\pred{orange}$, $\pred{pant}$, $\pred{paper}$, $\pred{phone}$, $\pred{pizza}$, $\pred{plant}$,  \\ $\pred{plate}$, $\pred{pole}$, $\pred{pot}$, $\pred{racket}$, $\pred{screen}$, $\pred{sheep}$, $\pred{shirt}$, $\pred{shoe}$, $\pred{short}$,  \\ $\pred{sign}$, $\pred{skateboard}$, $\pred{ski}$, $\pred{sneaker}$, $\pred{sock}$, $\pred{surfboard}$, $\pred{tie}$, $\pred{towel}$,  \\ $\pred{trunk}$, $\pred{umbrella}$, $\pred{vase}$, $\pred{vegetable}$, $\pred{wire}$, $\pred{zebra}$} \\ \hline
$\pred{thingsToSitOn}$ & 1 & \specialcell{$\pred{airplane}$, $\pred{beach}$, $\pred{bed}$, $\pred{bench}$, $\pred{bike}$, $\pred{boat}$, $\pred{branch}$, $\pred{bus}$, $\pred{car}$, $\pred{chair}$,  \\ $\pred{desk}$, $\pred{elephant}$, $\pred{horse}$, $\pred{motorcycle}$, $\pred{plane}$, $\pred{rock}$, $\pred{seat}$, $\pred{shelf}$,  \\ $\pred{sidewalk}$, $\pred{snow}$, $\pred{stand}$, $\pred{table}$, $\pred{train}$, $\pred{truck}$, $\pred{vehicle}$} \\ \hline
$\pred{toEat}$ & 1 & \specialcell{$\pred{banana}$, $\pred{food}$, $\pred{fruit}$, $\pred{orange}$, $\pred{pizza}$, $\pred{vegetable}$} \\ \hline
$\pred{transport}$ & 1 & \specialcell{$\pred{airplane}$, $\pred{bike}$, $\pred{boat}$, $\pred{bus}$, $\pred{car}$, $\pred{motorcycle}$, $\pred{plane}$, $\pred{train}$, $\pred{truck}$,  \\ $\pred{vehicle}$} \\ \hline
$\pred{transportHas}$ & 1 & \specialcell{$\pred{light}$, $\pred{seat}$, $\pred{wheel}$} \\ \hline
$\pred{treeOn}$ & 1 & \specialcell{$\pred{beach}$, $\pred{building}$, $\pred{hill}$, $\pred{mountain}$, $\pred{sidewalk}$, $\pred{snow}$, $\pred{street}$, $\pred{track}$,  \\ $\pred{tree}$} \\ \hline
$\pred{umbrellaS}$ & 2 & \specialcell{$\pred{carrying}$, $\pred{has}$, $\pred{holding}$, $\pred{of}$, $\pred{under}$, $\pred{with}$} \\ \hline
$\pred{walking}$ & 2 & \specialcell{$\pred{walking in}$, $\pred{walking on}$} \\ \hline
$\pred{wearingAll}$ & 2 & \specialcell{$\pred{has}$, $\pred{in}$, $\pred{on}$, $\pred{wearing}$, $\pred{wears}$, $\pred{with}$} \\ \hline
$\pred{wearingExact}$ & 2 & \specialcell{$\pred{wearing}$, $\pred{wears}$} \\ \hline

\end{tabular}
\caption{The third set of category definitions for the Visual Genome ontology.}
\label{table:categories3}
\end{table}
